# Supplementary material for: DyCON: Dynamic Uncertainty-aware Consistency and Contrastive Learning for Semi-supervised Medical Image Segmentation
Source: arXiv:2504.04566 source file (2025-04-06)
Supplement: Supplementary file 1 [file X_suppl.tex]

\clearpage
\setcounter{page}{1}
\maketitlesupplementary
This supplementary material is organized as follows:
\begin{itemize}
    \item \textbf{Appendix}~\ref{sec:datasets} provides more details about the datasets.
    \item \textbf{Appendix}~\ref{sec:gradient_analysis} provides the gradient analysis of UnCL loss function with loss surface and grad-cam visualizations.
    \item \textbf{Appendix}~\ref{sec:more_ablation} provides more ablation analysis of different properties of both loss functions.
    \item \textbf{Appendix}~\ref{sec:more_qualitative} provides more qualitative results from different datasets.    
    \item \textbf{Appendix}~\ref{sec:btcv_results} provides additional experiments on multi-organ segmentation task using BTCV dataset~\cite{btcv}.
    % \item \textbf{Appendix}~\ref{sec:pseudo_codes} provides the PyTorch codes for both UnCL and FeCL losses.
\end{itemize}
All of the above experimental analysis are conducted with a model trained using 10\% labeled data for both ISLES'22 and BraTS'19 datasets to ensure consistency.

\section{Datasets}
\label{sec:datasets}
\textbf{ISLES-2022:} The ISLES-2022 dataset~\cite{ISLES2022}\footnote{https://isles22.grand-challenge.org/isles22/} focuses on segmenting acute and sub-acute ischemic stroke lesions using 3D multi-channel MRI scans (DWI, ADC, and FLAIR). Unless otherwise specified, we use the DWI modality only, as it is highly sensitive to detecting acute ischemic lesions by excluding FLAIR due to registration complexities. The dataset consists of 250 skull-stripped cases (three cases \{150, 151, 170\} without lesion masks). We use 200 (80\%) images for training and the rest 50 (20\%) images for validation and testing. This dataset presents a challenge due to the small and scattered nature of stroke lesions, making it well-suited for evaluating DyCON's ability to handle uncertain and imbalanced regions. 

Fig.~\ref{fig:isles22_dataset} highlights the severe class imbalance in this dataset by revealing the distribution of lesion counts, sizes and scatterness. The figure emphasizes the challenge posed by the dominance of non-lesion and small lesions and the scarcity of large ones, which complicates model training and impacts segmentation performance. 
\begin{figure}[!ht]
    \centering
    \includegraphics[width=\linewidth]{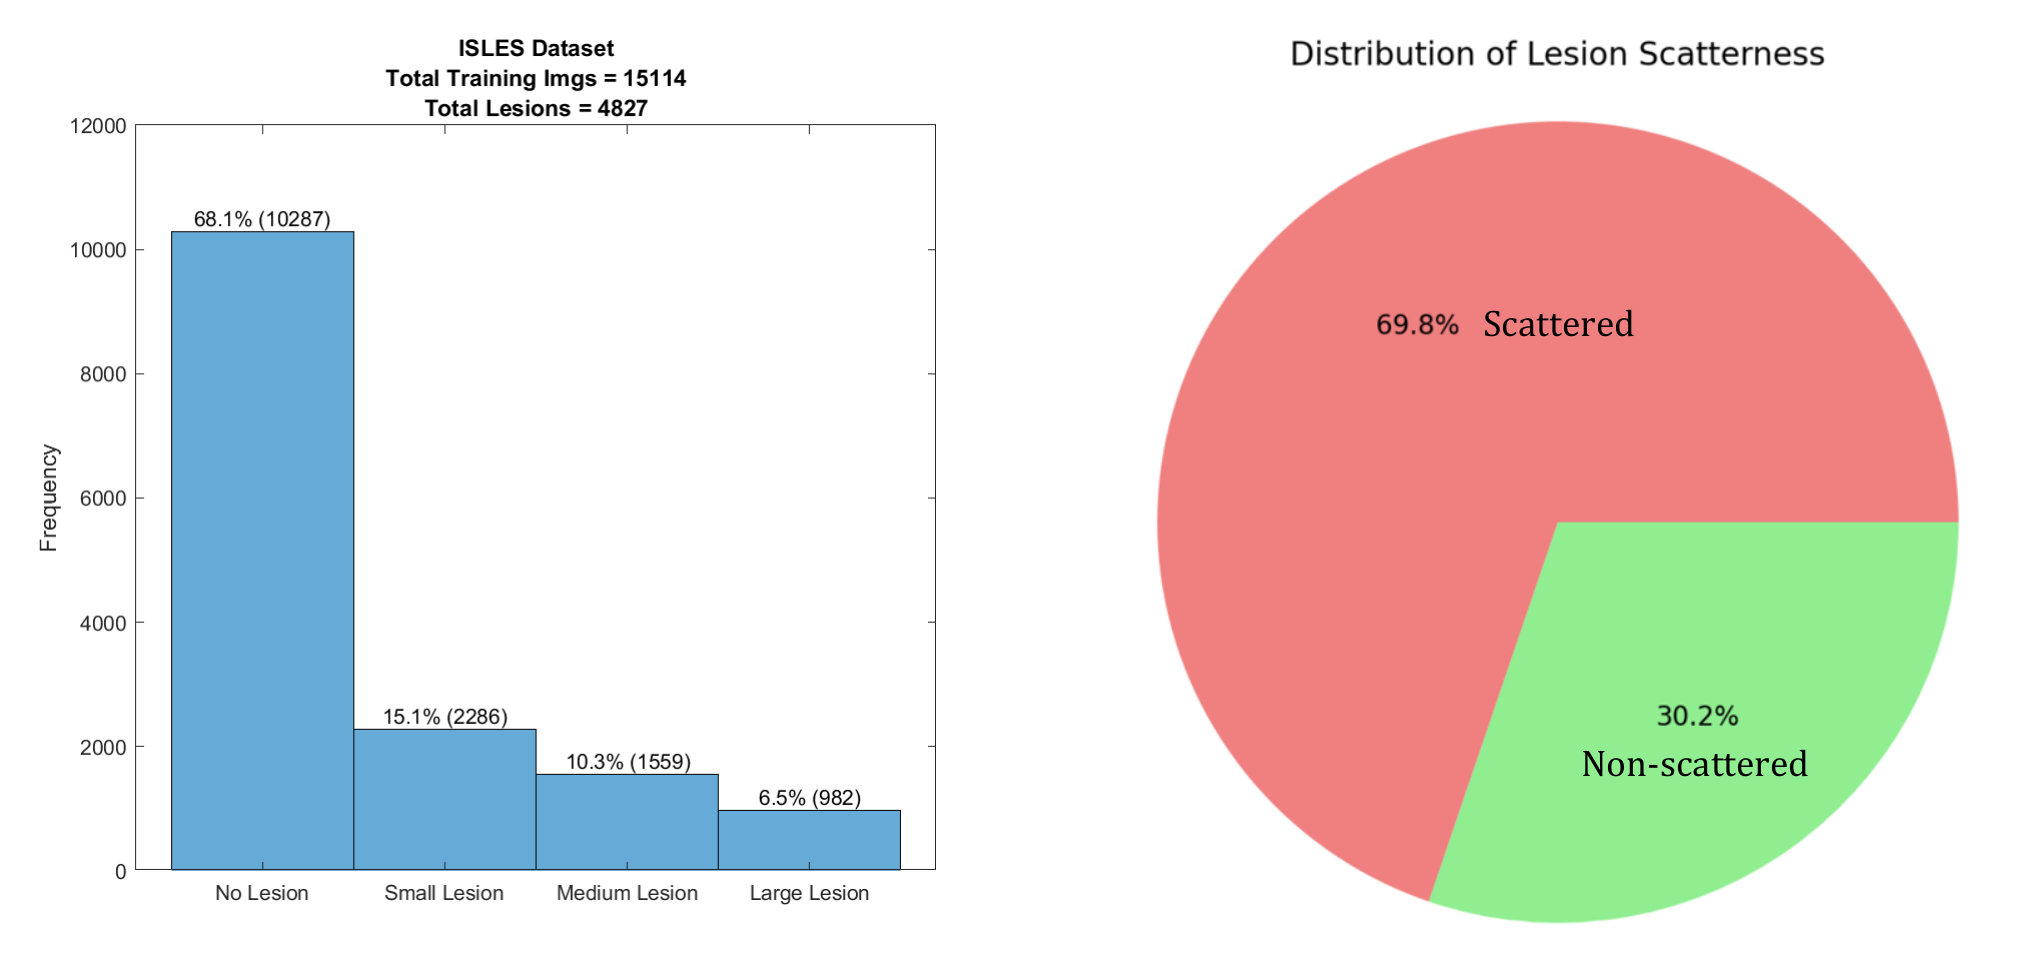}
    \caption{Characteristics of ISLES-2022 dataset. (Left) Lesion size distribution, and (Right) Lesion scatterness distribution.}
    \label{fig:isles22_dataset}
    \vspace{-1.2em}
\end{figure}

\textbf{BraTS2019:} The BraTS2019 dataset~\cite{brats2019} consists of 335 preoperative MRI scans (T1, T1ce, T2, T2-FLAIR) with annotations for brain tumors. We use the T2-FLAIR sequence for whole tumor segmentation, since it enhances the visibility of peritumoral edema critical for accurately capturing the entire tumor region. The dataset is split into 250/25/60 scans for training, validation, and testing. The focus of DyCON on uncertainty and contrastive learning is particularly valuable for this dataset, such as highly heterogeneous tumor regions, which poses challenges in segmentation.

\textbf{LA dataset:} The Left Atrium (LA) dataset~\cite{LA_dataset} includes 100 3D gadolinium-enhanced MRI (GE-MRIs) images with manually annotated left atrial segmentation masks. Each scan has an isotropic resolution of \(0.625\times 0.625\times 0.625mm^3\). Following~\cite{xu:ambiguity}, we used the 80/20 train/test split, with images cropped to the heart region and normalized to zero mean and unit variance. This dataset poses a class imbalance problem, with the left atrium occupying a small portion of the overall image.

\textbf{Pancreas-NIH:} The Pancreas-NIH dataset~\cite{Pancreas_dataset} comprises 82 3D CT images with pancreas annotations. For comparison, we follow split settings from BCP~\cite{bai:BCP}. This dataset is particularly challenging due to the pancreas's proximity to other organs and its unclear boundaries. DyCON's ability to adapt to uncertain regions makes it a strong candidate for accurate boundary delineation in this dataset.

\section{Gradient Analysis of UnCL Loss}
\label{sec:gradient_analysis}
According to the DyCON framework in Fig.2, the teacher model $f^t_\theta$ evolves via an EMA of the student model $f^s_\theta$, and only the student model is optimized using UnCL loss:
\begin{equation}
    \begin{aligned}
        \mathcal{L}_{\text{UnCL}} &= \frac{1}{N} \sum_{i=1}^{N} \frac{\mathcal{L}\left(p^s_i,p^t_i\right)}
        {\exp(\beta \cdot H_s(p^s_i)) + \exp(\beta \cdot H_t(p^t_i))} \\
        &\quad + \frac{\beta}{N} \sum_{i=1}^{N} \left(H_s(p^s_i) + H_t(p^t_i)\right)
    \end{aligned}
    \label{eq:l_UnCL}
\end{equation}
where: 
\begin{itemize}
    \item \( p^s = \sigma(f^s_\theta(x_j^s)) \) are the student predictions (trainable).
    \item \( p^t = \sigma(f^t_\theta(x_j^t)) \) are the teacher predictions (non-trainable).
    \item \( H_s(p^s_i) = -\sum_c p^s_{i,c} \log p^s_{i,c} \) is the entropy of the student predictions,
    \item \( H_t(p^t_i) = -\sum_c p^t_{i,c} \log p^t_{i,c} \) is the entropy of the teacher predictions,
    \item \(\beta > 0\) is a hyperparameter controlling the influence of entropy regularization.
\end{itemize}

\textbf{Gradient Computation:}
Since \( f^t_\theta \) is updated via EMA, the gradient computations focus solely on the student model \( f^s_\theta \). Therefore, the gradient of \(\mathcal{L}_{\text{UnCL}}\) with respect to the student model parameters \(\theta^s\) is:
\begin{equation}
    \resizebox{\columnwidth}{!}{
    $
    \begin{aligned}
        \frac{\partial \mathcal{L}_{\text{UnCL}}}{\partial \theta^s} = \frac{1}{N} \sum_{i=1}^{N} \Bigg[
        & \frac{\partial}{\partial \theta^s} \left( \frac{\mathcal{L}(p^s_i, p^t_i)}{\exp(\beta \cdot H_s(p^s_i)) + \exp(\beta \cdot H_t(p^t_i))} \right) \\
        & + \frac{\partial}{\partial \theta^s} \left( \beta H_s(p^s_i) \right) \Bigg].
    \end{aligned}
    $
    }
\end{equation}
The consistency loss term (\eg MSE) is defined as:
\begin{equation}
\mathcal{L}(p^s_i, p^t_i) = \|p^s_i - p^t_i\|^2.
\end{equation}
The gradient of \(\mathcal{L}(p^s_i, p^t_i)\) with respect to \(p^s_i\) is:
\begin{equation}
\frac{\partial \mathcal{L}(p^s_i, p^t_i)}{\partial p^s_i} = 2(p^s_i - p^t_i).
\end{equation}
Using the chain rule, the gradient with respect to \(\theta^s\) is:
\begin{equation}
\frac{\partial \mathcal{L}(p^s_i, p^t_i)}{\partial \theta^s} = 2(p^s_i - p^t_i) \cdot \frac{\partial p^s_i}{\partial \theta^s}.
\end{equation}
Therefore, the denominator \(\exp(\beta \cdot H_s(p^s_i)) + \exp(\beta \cdot H_t(p^t_i))\) inversely scales the gradient by predictive uncertainty. Its derivative with respect to \(\theta^s\) is:
% \begin{equation}
% \frac{\partial}{\partial \theta^s} \left( \exp(\beta \cdot H_s(p^s_i)) + \exp(\beta \cdot H_t(p^t_i)) \right) = \beta \exp(\beta \cdot H_s(p^s_i)) \frac{\partial H_s(p^s_i)}{\partial p^s_i} \frac{\partial p^s_i}{\partial \theta^s}.
% \end{equation}
\begin{equation}
\resizebox{\columnwidth}{!}{
$
\begin{aligned}
    \frac{\partial}{\partial \theta^s} \left( \exp(\beta \cdot H_s(p^s_i)) + \exp(\beta \cdot H_t(p^t_i)) \right) = 
    & \, \beta \exp(\beta \cdot H_s(p^s_i)) \\
    & \times \frac{\partial H_s(p^s_i)}{\partial p^s_i} \\
    & \times \frac{\partial p^s_i}{\partial \theta^s}.
\end{aligned}
$
}
\end{equation}
Here, the entropy gradient \(\frac{\partial H_s(p^s_i)}{\partial p^s_i}\) is:
\begin{equation}
\frac{\partial H_s(p^s_i)}{\partial p^s_{i,c}} = -(\log p^s_{i,c} + 1).
\end{equation}
Thus, the gradient of the consistency loss is modulated by both the alignment term \(p^s_i - p^t_i\) and the entropy-based scaling factor.

The second term 
% $\frac{\beta}{N} \sum_{i=1}^{N} \left(H_s(p^s_i) + H_t(p^t_i)\right)$, 
\(\frac{\beta}{N} \sum_{i=1}^{N} H_s(p^s_i)\) in Eq.(\ref{eq:l_UnCL}) involves only the student entropy:
\begin{equation}
\frac{\partial H_s(p^s_i)}{\partial p^s_{i,c}} = -(\log p^s_{i,c} + 1),
\end{equation}
and thus:
\begin{equation}
\frac{\partial}{\partial \theta^s} \left( H_s(p^s_i) \right) = \frac{\partial H_s(p^s_i)}{\partial p^s_i} \cdot \frac{\partial p^s_i}{\partial \theta^s}.
\end{equation}
As a result, this term encourages the student model to produce more confident predictions in unambiguous regions as training progresses. Overall, the gradient of \(\mathcal{L}_{\text{UnCL}}\) with respect to \(\theta^s\) is:
% \begin{equation}
%     \frac{\partial \mathcal{L}_{\text{UnCL}}}{\partial \theta^s} = 
%     \frac{1}{N} \sum_{i=1}^N \left[
%     \frac{
%     2(p^s_i - p^t_i) \cdot \frac{\partial p^s_i}{\partial \theta^s}
%     }{
%     \exp(\beta H_s(p^s_i)) + \exp(\beta H_t(p^t_i))
%     } 
%     - 
%     \frac{
%     \beta \cdot (p^s_i - p^t_i)^2 \cdot \exp(\beta H_s(p^s_i)) \cdot \frac{\partial H_s(p^s_i)}{\partial p^s_i} \cdot \frac{\partial p^s_i}{\partial \theta^s}
%     }{
%     \left(\exp(\beta H_s(p^s_i)) + \exp(\beta H_t(p^t_i))\right)^2
%     }
%     +
%     \beta \cdot \frac{\partial H_s(p^s_i)}{\partial p^s_i} \cdot \frac{\partial p^s_i}{\partial \theta^s}
%     \right].
% \end{equation}
\begin{equation}
\resizebox{\columnwidth}{!}{
$
\begin{aligned}
    \frac{\partial \mathcal{L}_{\text{UnCL}}}{\partial \theta^s} = 
    & \frac{1}{N} \sum_{i=1}^N \Bigg[
    \frac{2(p^s_i - p^t_i) \cdot \frac{\partial p^s_i}{\partial \theta^s}}{\exp(\beta H_s(p^s_i)) + \exp(\beta H_t(p^t_i))} \\
    & - \frac{\beta \cdot (p^s_i - p^t_i)^2 \cdot \exp(\beta H_s(p^s_i)) \cdot \frac{\partial H_s(p^s_i)}{\partial p^s_i} \cdot \frac{\partial p^s_i}{\partial \theta^s}}{\left(\exp(\beta H_s(p^s_i)) + \exp(\beta H_t(p^t_i))\right)^2} \\
    & + \beta \cdot \frac{\partial H_s(p^s_i)}{\partial p^s_i} \cdot \frac{\partial p^s_i}{\partial \theta^s}
    \Bigg].
\end{aligned}
$
}
\end{equation}

\textbf{Convergency Dynamics:} 
The teacher model \(f^t_\theta\) evolves as a smoothed EMA of the student model \(f^s_\theta\), acting as a stable reference. % The convergence dynamics are as follows:
\textbf{(a) Alignment with Teacher Predictions:} The gradient of \(\mathcal{L}_{\text{UnCL}}\) encourages the student predictions \(p^s\) to align with the teacher predictions \(p^t\), serving as a denoised target. \textbf{(b) Uncertainty Focus:} The exponentiated entropy-based weighting \(\exp(\beta \cdot H_s(p^s_i)) + \exp(\beta \cdot H_t(p^t_i))\) focuses the optimization on regions with high uncertainty, such as lesion boundaries. \textbf{(c) Confidence Calibration:} The entropy regularization term \(\frac{\beta}{N} \sum_{i=1}^N H_s(p^s_i)\) prevents overconfidence, promoting generalization.

\textbf{Implications for Medical Image Segmentation:} \textbf{(a) Boundary Refinement:} High-entropy regions (e.g., lesion boundaries) are emphasized during optimization to improve segmentation accuracy.
% \textbf{(b) Noise Robustness:} The EMA-smoothed teacher model provides a stable target to reduce noise sensitivity. 
\textbf{(b) Generalization:} The combination of alignment and uncertainty regularization ensures the model balances sharpness and coverage in segmentation.
% \textbf{Convergency Dynamics:} 
% The teacher model \(f^t_\theta\) evolves as a smoothed EMA of the student model \(f^s_\theta\), acting as a stable reference. The convergence dynamics are as follows:
% \begin{itemize}
%     \item \textbf{Alignment with Teacher Predictions:} The gradient of \(\mathcal{L}_{\text{UnCL}}\) encourages the student predictions \(p^s\) to align with the teacher predictions \(p^t\), serving as a denoised target. 
%     \item \textbf{Uncertainty Focus:} The exponentiated entropy-based weighting \(\exp(\beta \cdot H_s(p^s_i)) + \exp(\beta \cdot H_t(p^t_i))\) focuses the optimization on regions with high uncertainty, such as lesion boundaries. 
%     \item \textbf{Confidence Calibration:} The entropy regularization term \(\frac{\beta}{N} \sum_{i=1}^N H_s(p^s_i)\) prevents overconfidence, promoting generalization.
% \end{itemize}

% \textbf{Implications for Medical Image Segmentation:} 
% \begin{itemize}
%     \item \textbf{Boundary Refinement:} High-entropy regions (e.g., lesion boundaries) are emphasized during optimization to improve segmentation accuracy. 
%     % \item \textbf{Noise Robustness:} The EMA-smoothed teacher model provides a stable target to reduce noise sensitivity. 
%     \item \textbf{Generalization:} The combination of alignment and uncertainty regularization ensures the model balances sharpness and coverage in segmentation results.
% \end{itemize}

\subsection{Loss Surface Visualization}
\label{subsec:loss_surface}
Fig.~\ref{fig:loss_surface} illustrates the loss surface visualization over course of training on ISLES-22 and BraTS-19 datasets, which highlights the dynamics of UnCL's optimization process. The sharp spikes and valleys indicate regions of high uncertainty, corresponding to ambiguous areas such as subtle lesion boundaries or scattered lesions. By leveraging dual-entropy from both teacher and student models, UnCL dynamically modulates the consistency loss in these regions, mitigating the impact of noisy gradients and overconfident predictions. This results in a smoother and more balanced optimization trajectory, promoting stability and better segmentation accuracy in complex lesion distributions. 
\begin{figure}[!ht]
    \centering
    \includegraphics[width=\linewidth]{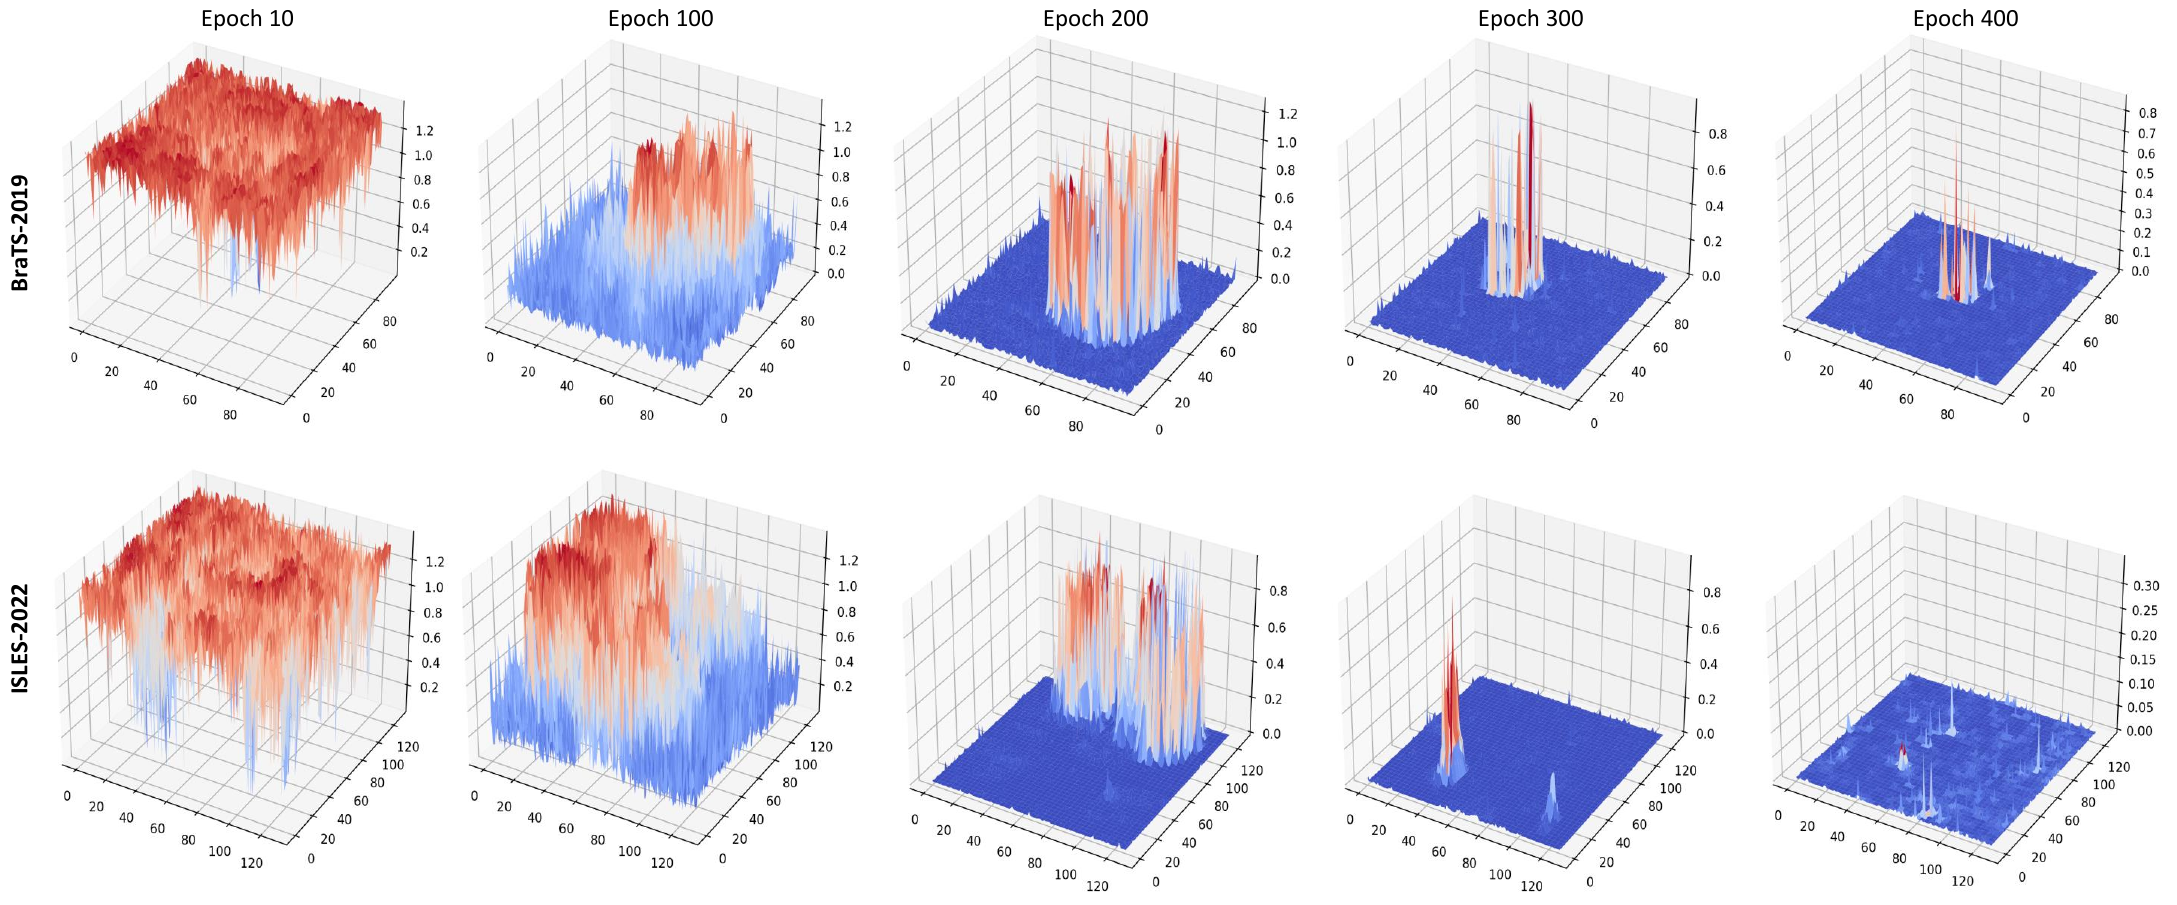}
    \caption{Loss landscape visualization of UnCL loss over training epochs for samples in ISLES'22 and BraTS'19 datasets. Notably, the loss surface is steadily converging toward better alignment and lower uncertainty across both datasets.}
    \label{fig:loss_surface}
\end{figure}

% \begin{equation}
%     \resizebox{\columnwidth}{!}{
%         $\begin{aligned}
%             % \frac{\partial \mathcal{L}_{\beta\text{MSE}}}{\partial p^s}
%             \nabla_{p_j^s}\mathcal{L}_{\beta\text{MSE}}
%             &= \frac{2(p_j^s - p_j^t)}{\exp(\beta \cdot H_s(p_j^s)) + \exp(\beta \cdot H_t(p_j^t))} \\
%             &\quad - \frac{(p_j^s - p_j^t)^2 \cdot \beta \cdot \frac{\partial H_s(p_j^s)}{\partial p_j^s} \cdot \exp(\beta \cdot H_s(p_j^s))}{\left(\exp(\beta \cdot H_s(p_j^s)) + \exp(\beta \cdot H_t(p_j^t))\right)^2}
%         \end{aligned}$
%     }
%     \label{eqn:grad_weighted_mse}
% \end{equation}

\subsection{Grad-CAM Visualization}
\label{subsec:more_grad_cams}
In this section, we visualize class-wise activation maps from the penultimate decoder layer of 3D-UNet to further gain interpretable insights into the inherent properties of UnCL loss as shown in Fig.\ref{fig:grad_cam}. The Grad-CAM visualizations effectively highlight DyCON's capability to focus on uncertain regions over the course of training. In early epochs (100), the heatmaps show a broader and less focused activation across the brain, indicating high uncertainty in identifying lesion regions, aligned to the ground truth masks. As training progresses (late 400 epochs), the activations become more refined and concentrated around the true lesion areas. This refinement reflects the model's robustness to accurately localize and segment subtle lesions, enhancing lesion boundary precision and overall segmentation accuracy.
\vspace{-1.5em}
\begin{figure}[!t]
  \centering
  % \fbox{\rule{0pt}{2in} \rule{0.9\linewidth}{0pt}}
   \includegraphics[width=\linewidth]{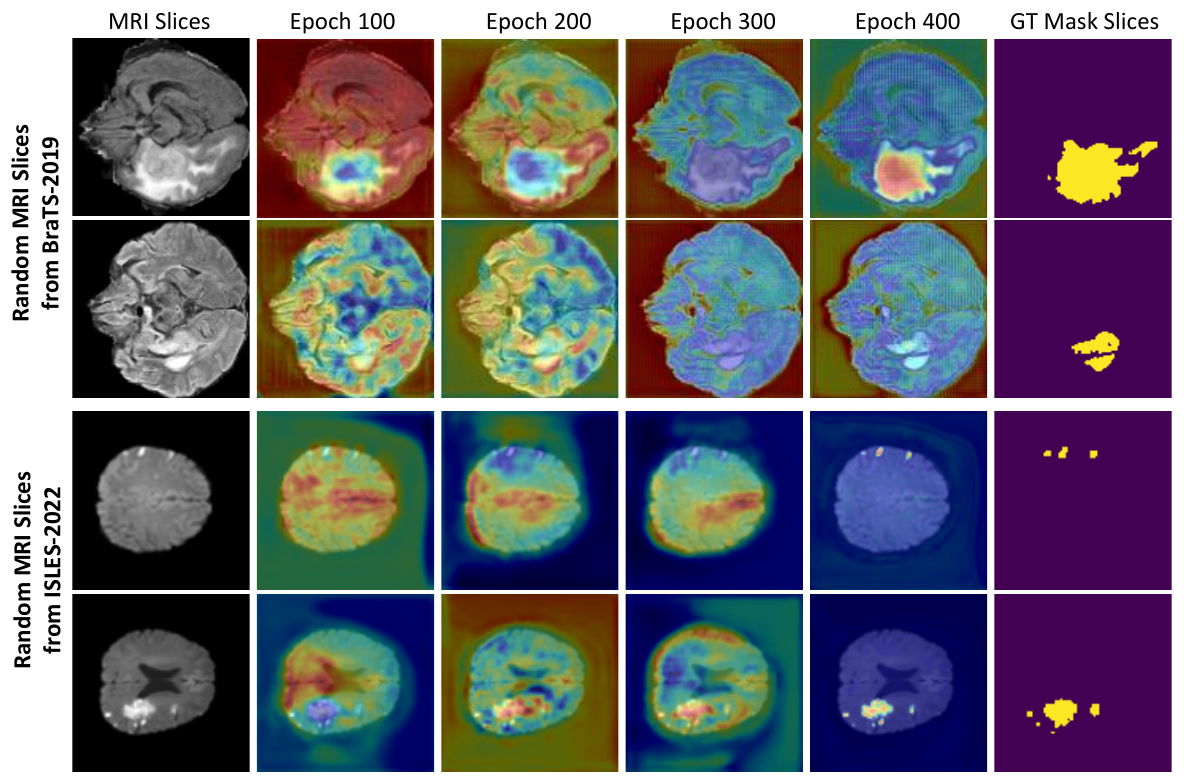}
   \caption{ Grad-CAM visualizations over training epochs on ISLES'22 and BraTS'19 datasets. Progressively, the model's attention focuses on lesion regions, showing improved alignment with ground truth masks as training progresses.}
   \label{fig:grad_cam}
   \vspace{-1.5em}
\end{figure}
% The consistent improvement in focus and localization observed through these heatmaps complements the gradient magnitude analysis. Thus, driven by $\beta$MSE DyCON effectively prioritizes uncertain regions early on and gradually shifts to more confident predictions. This dynamic approach enhances lesion boundary precision and overall segmentation accuracy.

\section{More Ablation Study}
\label{sec:more_ablation}
\subsection{The Essence of Dual-entropy in UnCL Loss}
\label{subsec:effect_of_dual_entropy}
In this subsection, we analyze the role of dual-entropy (entropy from student and teacher models) in enhancing the performance of the UnCL loss. Dual-entropy introduces a principled mechanism for jointly capturing uncertainty from both models, which proves particularly effective in lesion segmentation under class imbalance and variability. Specifically, we trained DyCON with single-entropy from the teacher and student models without modifying other components. Table~\ref{tab:dual_entropy} highlights the performance improvement of using dual-entropy over single-entropy baselines on the ISLES-22 dataset. For example, the Dice score improves from 63.14\% (teacher entropy only) and 64.42\% (student entropy only) to 65.75\% with dual-entropy. This result reflects the importance of leveraging uncertainties from both models. 
% Similar trends are observed across other datasets, underscoring the importance of leveraging uncertainties from both models. 
\begin{table}[!t]
    \centering
    \resizebox{\columnwidth}{!}{
    \begin{tabular}{lllll}
    \toprule
    Strategy        & Dice (\%) & IoU (\%) & HD95$\downarrow$ & ASD$\downarrow$ \\
    \midrule
    Teacher-Entropy & 63.14   & 48.85    &  15.23    & 2.15    \\
    Student-Entropy & 64.42   & 50.24    &  14.25    & 1.64    \\
    Dual-Entropy    & 65.75   & 51.20    &  13.30    & 0.76    \\
    \bottomrule
    \end{tabular}
    }
    \caption{The effect of using single-entropy and dual-entropy in UnCL loss using 10\% labeled data.}
    \label{tab:dual_entropy}
    % \vspace{-1em}
\end{table}
\begin{figure}[!t]
    \centering
    \includegraphics[width=8cm, height=7cm]{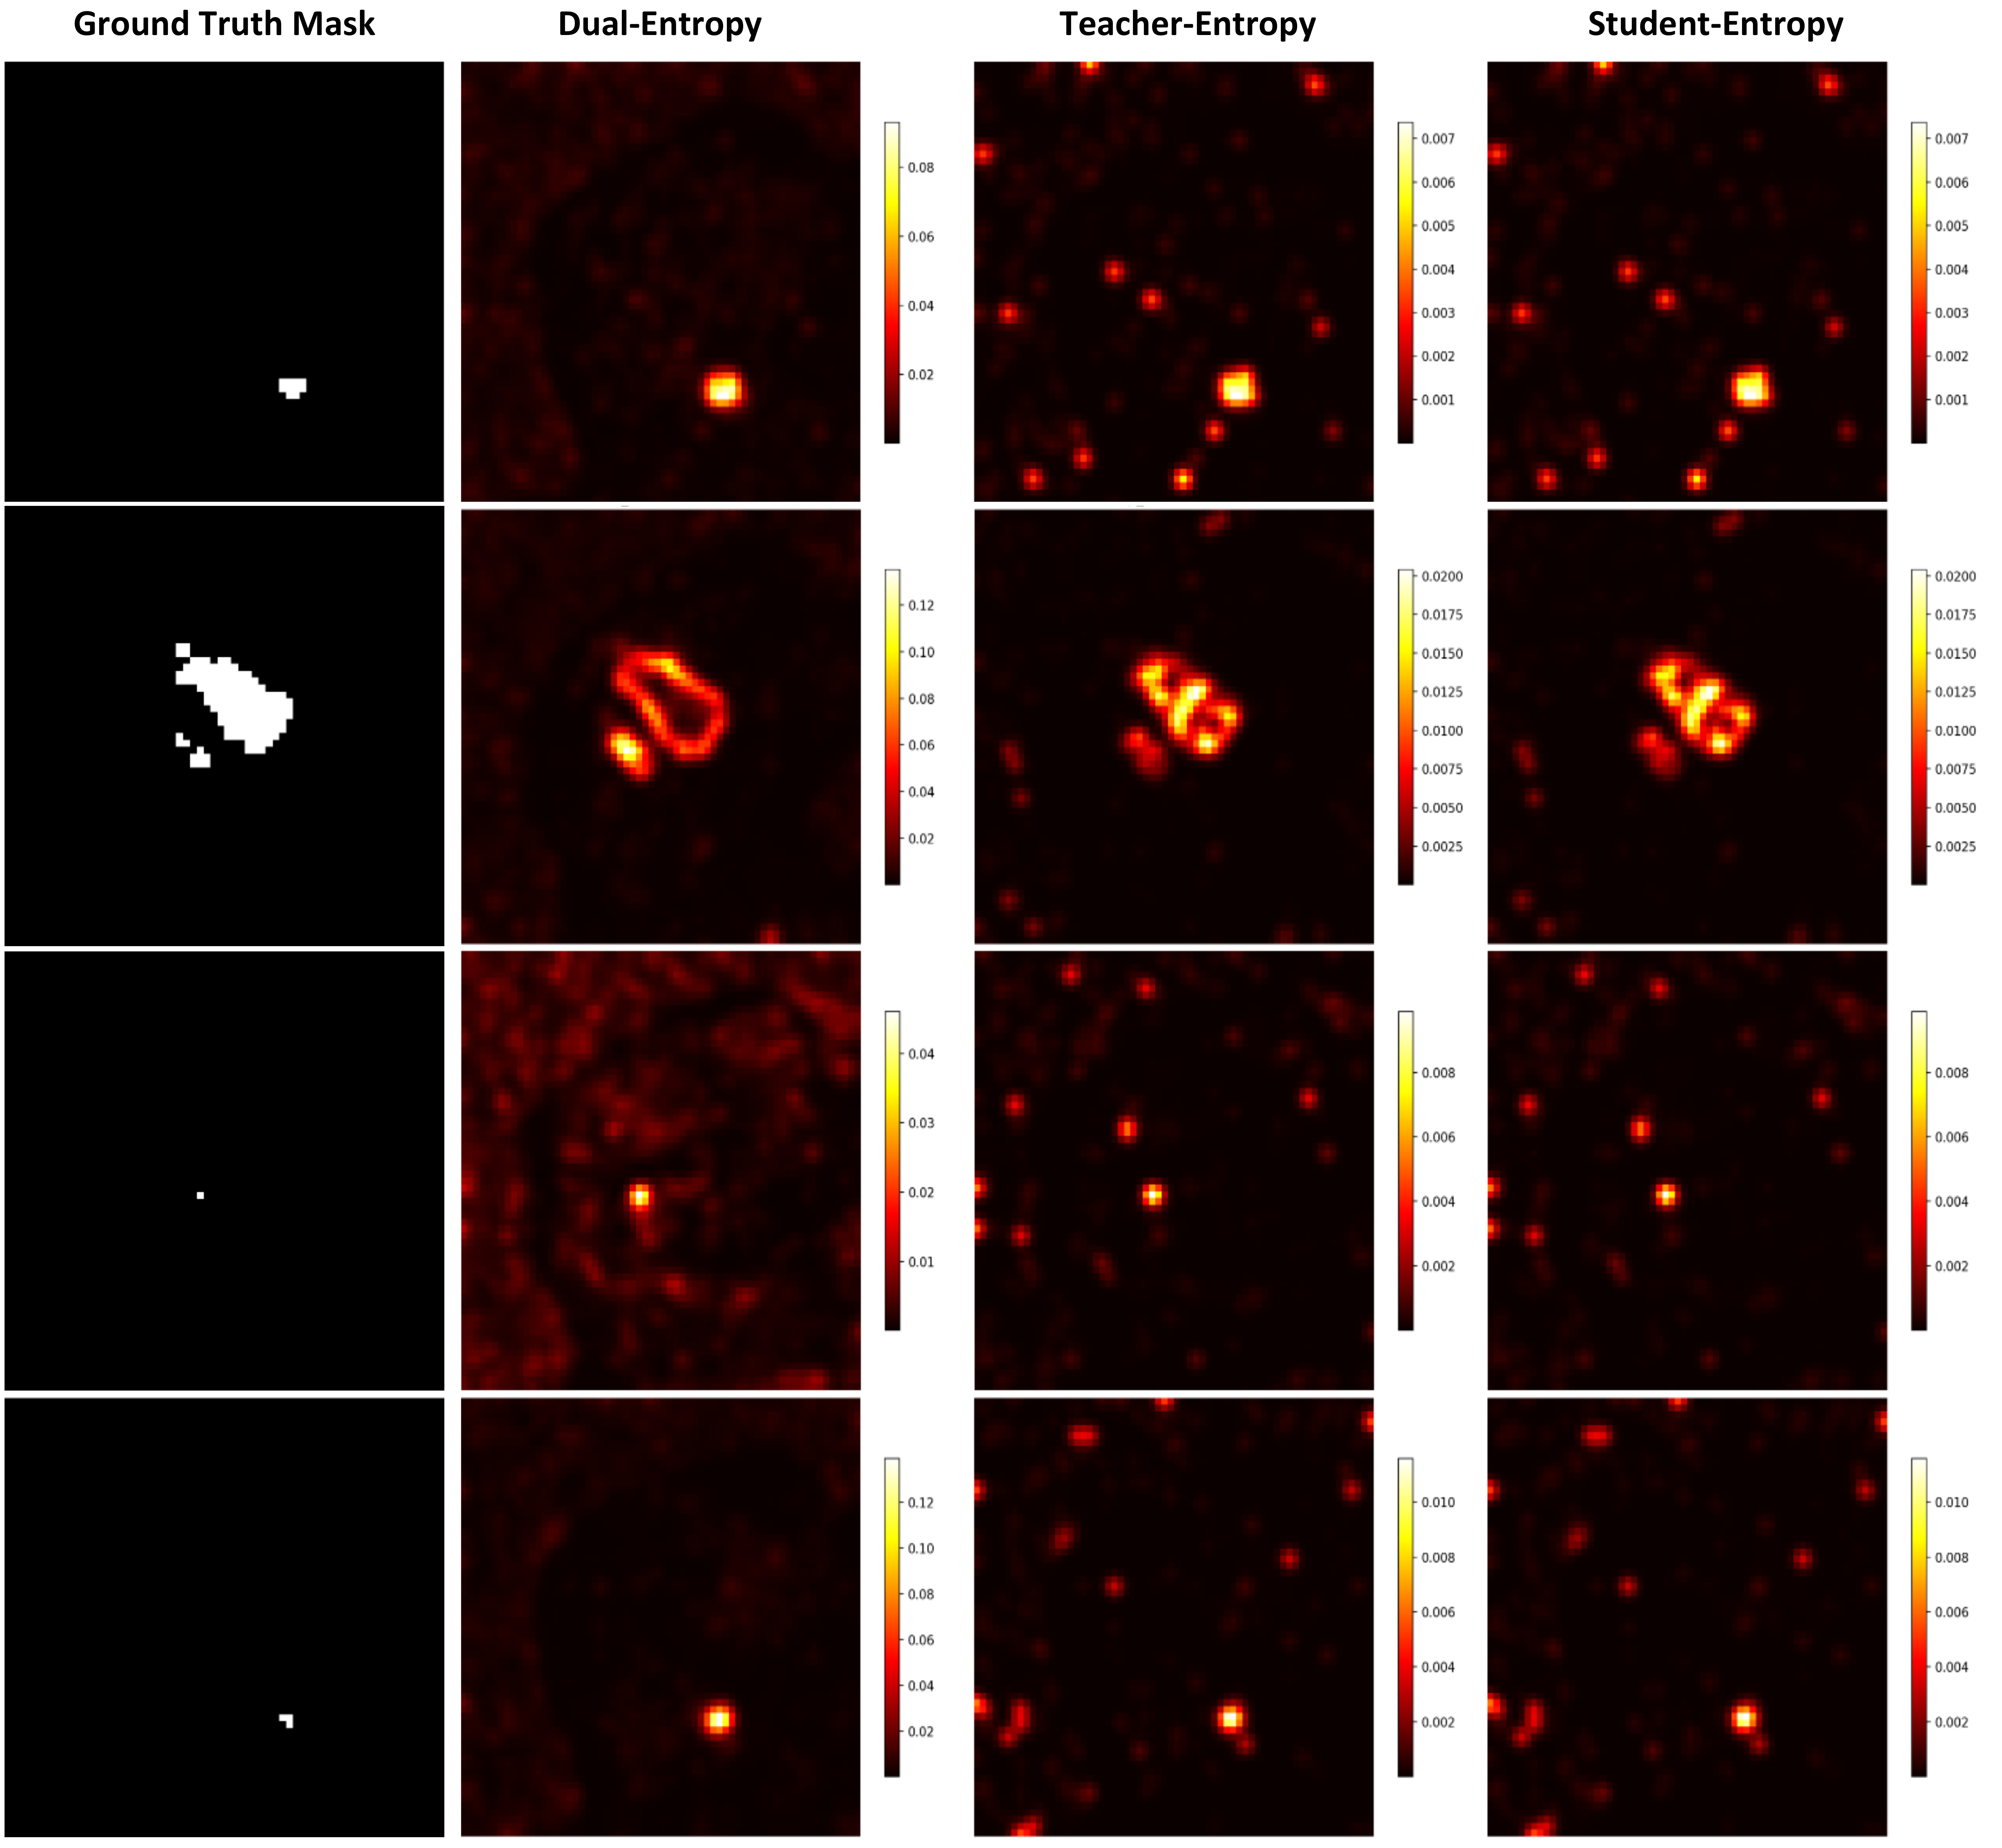}
    \caption{ Illustration of uncertainty maps generated using dual-entropy and single-entropy strategies from the teacher and student models in UnCL Loss.}
    \label{fig:dual_entropy}
    \vspace{-1.2em}
\end{figure}

Fig.~\ref{fig:dual_entropy} further demonstrates the impact of single-entropy and dual-entropy strategies when combined with the UnCL loss. The visualizations reveal that relying solely on either teacher or student entropy results in overconfident predictions in regions of high ambiguity, such as small lesions. It struggle to reduce uncertainty, exhibiting higher noise levels while still vaguely highlighting ground truth regions. This overconfidence occurs because a single-entropy approach fails to adequately capture the uncertainty inherent in such challenging areas. In contrast, the dual-entropy effectively reduces uncertainty over challenging lesion regions, as seen by the sharper focus around ground truth areas with minimal noise. This shows that dual-entropy provides more stable and precise guidance, improving the model's confidence and segmentation performance in ambiguous areas.

\subsection{Effects of Hyperparameters in FeCL}
\label{subsec:inter_intra_net}
To analyze the impact of the focal weighting factor $\gamma$ and the top-$k$ hard negative selection in FeCL, we conduct a detailed ablation study across two datasets, focusing on their respective roles in improving lesion segmentation performance. These parameters are crucial in addressing class imbalance and enhancing the model's ability to discriminate subtle lesion boundaries under challenging conditions.

\textbf{Effect of Focus Controller $\gamma$:}
The parameter $\gamma$ modulates the contribution of hard positive and negative patch pairs by emphasizing samples that are difficult to distinguish. A higher $\gamma$ value increases the weight on hard-to-distinguish patch pairs, while lower values reduce the emphasis, treating all samples more uniformly. In this experiment, we vary $\gamma\in \{0.5, 0.8, 1.0, 1.5, 2.0\}$ and evaluate segmentation accuracy using Dice and HD95 metrics. All experiments are conducted on both datasets with 10\% labeled data, keeping the other FeCL components constant. The results for various $\gamma$ are reported in Fig.~\ref{fig:lambda_comparison}. 

The focal weighting factor $\gamma$ in FeCL demonstrates optimal performance at $\gamma=0.8$ for BraTS'19 and $\gamma=0.5$ for ISLES'22, achieving a balance between emphasizing hard positive and negative patch pairs and avoiding over-amplification of noise. Increasing $\gamma$ beyond this value leads to %diminishing returns, with only 
marginal performance improvements, which indicates the model already effectively captures complex lesion characteristics with moderate $\gamma$, such as variability in size, shape, and spatial distribution. This phenomenon highlights the robustness of FeCL to lesion complexity in handling small, irregular, and scattered lesions. The results suggest that $\gamma=\{0.8, 0.5\}$ provides the optimal trade-off between emphasizing subtle lesion patterns and maintaining training stability. In this way, FeCL ensures consistent feature discrimination across diverse and challenging datasets.
% For precise positioning, use the legend style option and specify at={(x,y)}. The coordinates (x,y) are normalized such that (0,0) is the bottom-left and (1,1) is the top-right of the plot.
\begin{figure}[!t]
    \centering
    % Plot for Dice values
    \begin{subfigure}[t]{0.4\textwidth}
        \centering
        \begin{tikzpicture}
            \begin{axis}[
                axis x line=bottom,
                axis y line=left,
                tick pos=bottom,
                ytick pos=left,
                width=\textwidth,
                height=0.6\textwidth,       
                xlabel={$\gamma$},
                ylabel={Dice Score (\%)},
                legend style={at={(0.48,0.69)}, anchor=north west}, % Outside top-right
                grid=major,
                xtick={0.5, 0.8, 1, 1.5, 2},
                ymin=60, ymax=90,
                nodes near coords,
                nodes near coords style={font=\footnotesize}, % Tiny font for node labels
                xticklabel style={font=\footnotesize},
                every node near coord/.append style={font=\footnotesize} % Tiny font for nodes
                ]
                % Dice values for ISLES-2022
                \addplot[smooth, mark=*, blue] 
                coordinates {
                    (0.5, 65.71)
                    (0.8, 65.30)
                    (1, 64.02)
                    (1.5, 65.23)
                    (2, 64.78)
                };
                \addlegendentry{ISLES-2022}
                % Dice values for BraTS-2019
                \addplot[smooth, mark=square*, red] 
                coordinates {
                    (0.5, 86.34)
                    (0.8, 87.05)
                    (1, 86.8)
                    (1.5, 85.11)
                    (2, 83.67)
                };
                \addlegendentry{BraTS-2019}
            \end{axis}
        \end{tikzpicture}
    \end{subfigure}
    % \hfill
    % Plot for HD95 values
    \begin{subfigure}[t]{0.4\textwidth}
        \centering
        \begin{tikzpicture}
            \begin{axis}[
                axis x line=bottom,
                axis y line=left,
                tick pos=bottom,
                ytick pos=left,
                width=\textwidth,
                height=0.6\textwidth,  
                xlabel={$\gamma$},
                ylabel={HD95 (mm)},
                legend style={at={(0.70,0.76)}, anchor=north}, % Below the plot, centered
                grid=major,
                xtick={0.5, 0.8, 1, 1.5, 2},
                ymin=7, ymax=15,
                nodes near coords,
                nodes near coords style={font=\footnotesize}, % Tiny font for node labels
                xticklabel style={font=\footnotesize},
                every node near coord/.append style={font=\footnotesize} % Tiny font for nodes
                ]
                % HD95 values for ISLES-2022
                \addplot[smooth, mark=*, blue] 
                coordinates {
                    (0.5, 13.2)
                    (0.8, 13.28)
                    (1, 13.74)
                    (1.5, 13.49)
                    (2, 13.66)
                };
                \addlegendentry{ISLES-2022}
                % HD95 values for BraTS-2019
                \addplot[smooth, mark=square*, red] 
                coordinates {
                    (0.5, 7.81)
                    (0.8, 7.4)
                    (1, 7.55)
                    (1.5, 8.04)
                    (2, 9.13)
                };
                \addlegendentry{BraTS-2019}
            \end{axis}
        \end{tikzpicture}
    \end{subfigure}
    \vspace{-1em}
    \caption{Performance comparison of Dice scores and HD95 values for ISLES'22 and BraTS'19 datasets across different $\lambda$ values.}
    \label{fig:lambda_comparison}
    \vspace{-1.2em}
\end{figure}

\textbf{Effect of Top-$k$ Hard Negative Selection:}
The top-$k$ parameter controls the number of hard negatives incorporated from the teacher model, enriching the negative sampling process in the contrastive loss. In this experiment, we test $K\in\{8, 16, 24, 32\}$ while keeping the optimal values of \(\lambda\) fixed for BraTS-2019 and ISLES-2022 datasets. For each setting, we measure Dice and HD95 to evaluate segmentation performance. Fig.~\ref{fig:k_performance_comparison} shows the Dice and HD95 scores of various $K$ values. The key observations reveal that increasing $k$ up to $k=16$ enhances the diversity of negative samples, improving feature separability and segmentation performance, as evidenced by a Dice score increase from 63.57\% ($k$=8) to 65.71\% ($k$=16) on ISLES-22. Beyond $k$=16, the performance plateaus or slightly decreases across both datasets due to the inclusion of redundant or overly similar negatives, which introduces noise into the loss.
\begin{figure}[!t]
    \centering
    % Plot for Dice values
    \vspace{-1em}
    \begin{subfigure}[t]{0.4\textwidth}
        \centering
        \begin{tikzpicture}
            \begin{axis}[
                axis x line=bottom,
                axis y line=left,
                tick pos=bottom,
                ytick pos=left,
                width=\textwidth,
                height=0.6\textwidth,
                xlabel={$K$},
                ylabel={Dice Score (\%)},
                legend style={at={(0.48,0.68)}, anchor=north west}, % Outside top-right
                grid=major,
                xtick={8, 16, 24, 32},
                ymin=60, ymax=90,
                nodes near coords,
                nodes near coords style={font=\tiny}, % Tiny font for node labels
                xticklabel style={font=\footnotesize},
                every node near coord/.append style={font=\tiny} % Ensure all node fonts are tiny
                ]
                % Dice values for ISLES-2022
                \addplot[smooth, mark=*, blue] 
                coordinates {
                    (8, 63.57)
                    (16, 65.71)
                    (24, 64.42)
                    (32, 62.53)
                };
                \addlegendentry{ISLES-2022}

                % Dice values for BraTS-2019
                \addplot[smooth, mark=square*, red] 
                coordinates {
                    (8, 85.82)
                    (16, 87.1)
                    (24, 86.54)
                    (32, 84.34)
                };
                \addlegendentry{BraTS-2019}
            \end{axis}
        \end{tikzpicture}
    \end{subfigure}
    % \hfill
    % Plot for HD95 values
    \begin{subfigure}[t]{0.4\textwidth}
        \centering
        \begin{tikzpicture}
            \begin{axis}[
                axis x line=bottom,
                axis y line=left,
                tick pos=bottom,
                ytick pos=left,
                width=\textwidth,
                height=0.6\textwidth,
                xlabel={$K$},
                ylabel={HD95 (mm)},
                legend style={at={(0.72,0.7)}, anchor=north}, % Below the plot, centered
                grid=major,
                xtick={8, 16, 24, 32},
                ymin=7, ymax=15,
                nodes near coords,
                nodes near coords style={font=\tiny}, % Tiny font for node labels
                xticklabel style={font=\footnotesize},
                every node near coord/.append style={font=\tiny} % Ensure all node fonts are tiny
                ]
                % HD95 values for ISLES-2022
                \addplot[smooth, mark=*, blue] 
                coordinates {
                    (8, 14.12)
                    (16, 13.35)
                    (24, 13.63)
                    (32, 14.46)
                };
                \addlegendentry{ISLES-2022}

                % HD95 values for BraTS-2019
                \addplot[smooth, mark=square*, red] 
                coordinates {
                    (8, 7.93)
                    (16, 7.41)
                    (24, 7.62)
                    (32, 8.04)
                };
                \addlegendentry{BraTS-2019}
            \end{axis}
        \end{tikzpicture}
    \end{subfigure}
    \vspace{-1em}
    \caption{Performance comparison of Dice and HD95 values for ISLES-2022 and BraTS-2019 datasets across different $K$ values.}
    \label{fig:k_performance_comparison}
    \vspace{-1.2em}
\end{figure}

\subsection{Integrating DyCON with SSL Frameworks}
\label{subsec:integrate_dycon}
To demonstrate the versatility and effectiveness of DyCON, we integrate it into two representative semi-supervised learning frameworks: Mean-Teacher (MT)\cite{mean_teacher} and Co-training (CT)\cite{chen:semi_cross_pseudo_label}. These frameworks utilize distinct mechanisms for leveraging unlabeled data, providing a robust foundation for evaluating the adaptability of DyCON. 

In this regard, MT leverages a student-teacher paradigm where DyCON's UnCL improves global consistency by dynamically weighting uncertain regions, while FeCL enhances local feature discrimination for nuanced lesion segmentation, addressing class imbalance effectively. Similarly, Co-Training benefits from DyCON by using UnCL to align predictions from independent sub-networks through dual-entropy, and FeCL to refine local features, capturing subtle lesion details. DyCON significantly improves the performance of both frameworks on ISLES'22 and BraTS'19 datasets.

Our experiments demonstrate that DyCON consistently improves both MT and CT frameworks, as shown in Fig.~\ref{fig:dycon_with_mt_ct}. By enhancing global and local feature consistency, DyCON achieves superior segmentation results without requiring modifications to the underlying architectures. These findings highlight DyCON's adaptability and potential for broad adoption in SSL-based medical image segmentation.
\begin{figure}[!t]
    \centering
    % First histogram
    \begin{subfigure}[t]{0.48\textwidth}
        \centering
        \begin{tikzpicture}
            \begin{axis}[
                ybar=0pt,
                bar width=0.65cm,
                width=7cm,
                height=5cm,
                ymin=0,
                ymax=96,
                ylabel={Performance},
                symbolic x coords={MT, CT, MT+DyCON, {CT+DyCON}},
                xtick=data,
                x=1.65cm,
                nodes near coords,
                nodes near coords style={font=\small},
                enlarge x limits=0.2,
                legend style={at={(0.26,0.86)}, anchor=north, legend columns=-1},
                ylabel style={yshift=-0.5em},
                axis y line*=left,
                axis x line*=bottom,
                ymajorgrids=true,
                grid style=dashed,
                xticklabel style={font=\footnotesize},
                every node near coord/.append style={font=\footnotesize}
            ]
            % Dice scores (light skyblue)
            \addplot[draw=none, fill={rgb,255:red,135; green,206; blue,250}] coordinates {
                (MT, 36.43) (CT, 42.96) (MT+DyCON, 65.71) (CT+DyCON, 60.48)
            };
            % HD95 scores (light salmon)
            \addplot[draw=none, fill={rgb,255:red,250; green,128; blue,114}] coordinates {
                (MT, 21.8) (CT, 42.82) (MT+DyCON, 13.35) (CT+DyCON, 28.67)
            };
            \legend{Dice(\%)$\uparrow$, HD95$\downarrow$}
            \end{axis}
        \end{tikzpicture}
        \caption{ISLES'22 Results.}
        % \label{fig:isles22_results}
    \end{subfigure}
    % \hfill
    % Second histogram
    \begin{subfigure}[t]{0.48\textwidth}
        \centering
        \begin{tikzpicture}
            \begin{axis}[
                ybar=0pt,
                bar width=0.65cm,
                width=7cm,
                height=5cm,
                ymin=0,
                ymax=95,
                symbolic x coords={MT, CT, MT+DyCON, {CT+DyCON}},
                xtick=data,
                x=1.65cm,
                ylabel={Performance},
                nodes near coords,
                nodes near coords style={font=\small},
                enlarge x limits=0.2,
                legend style={at={(0.7,0.8)}, anchor=north, legend columns=-1},
                axis y line*=left,
                axis x line*=bottom,
                ymajorgrids=true,
                grid style=dashed,
                xticklabel style={font=\footnotesize},
                every node near coord/.append style={font=\footnotesize}
            ]
            % Dice scores (light skyblue)
            \addplot[draw=none, fill={rgb,255:red,135; green,206; blue,250}] coordinates {
                (MT, 81.7) (CT, 83.67) (MT+DyCON, 87.05) (CT+DyCON, 86.98)
            };
            % HD95 scores (light salmon)
            \addplot[draw=none, fill={rgb,255:red,250; green,128; blue,114}] coordinates {
                (MT, 22.29) (CT, 12.58) (MT+DyCON, 7.41) (CT+DyCON, 10.14)
            };
            \legend{Dice(\%)$\uparrow$, HD95$\downarrow$}
            \end{axis}
        \end{tikzpicture}
        \caption{BraTS'19 Results.}
        % \label{fig:brats19_results}
    \end{subfigure}
    \vspace{-0.5em}
    \caption{Comparative performance (Dice (\%) and HD95) when integrating DyCON into MT and CT frameworks with 10\% labeled data. DyCON enhances segmentation accuracy consistently across ISLES'22 and BraTS'19 datasets without modifying the underlying architectures or training pipelines.}
    \label{fig:dycon_with_mt_ct}
    \vspace{-1.2em}
\end{figure}
\vspace{-1.5em}
\section{More Visualization Results}
\label{sec:more_qualitative}
Fig.~\ref{fig:brats_and_isles_visualization} presents brain tumor and lesion segmentation visualizations from BraTS'19 and ISLES'22 datasets. Moreover, Fig.~\ref{fig:la_visualization} illustrates left atrium organ segmentation visualizations from LA dataset. These results demonstrate that, DyCON persistently delivers more accurate segmentation of complex lesions and organs compared to the SOTA methods across all datasets. Closely note that, in each of the visualizations the False Negatives (blues) are produced due to invariance of the lesion or tumor boundaries with the healthy tissues. In this case, DyCON has achieved a remarkable delineation of these challenging tumors and lesions regardless of their morphological difficulties.
\begin{figure}[!ht]
    \centering
    \includegraphics[width=8.5cm]{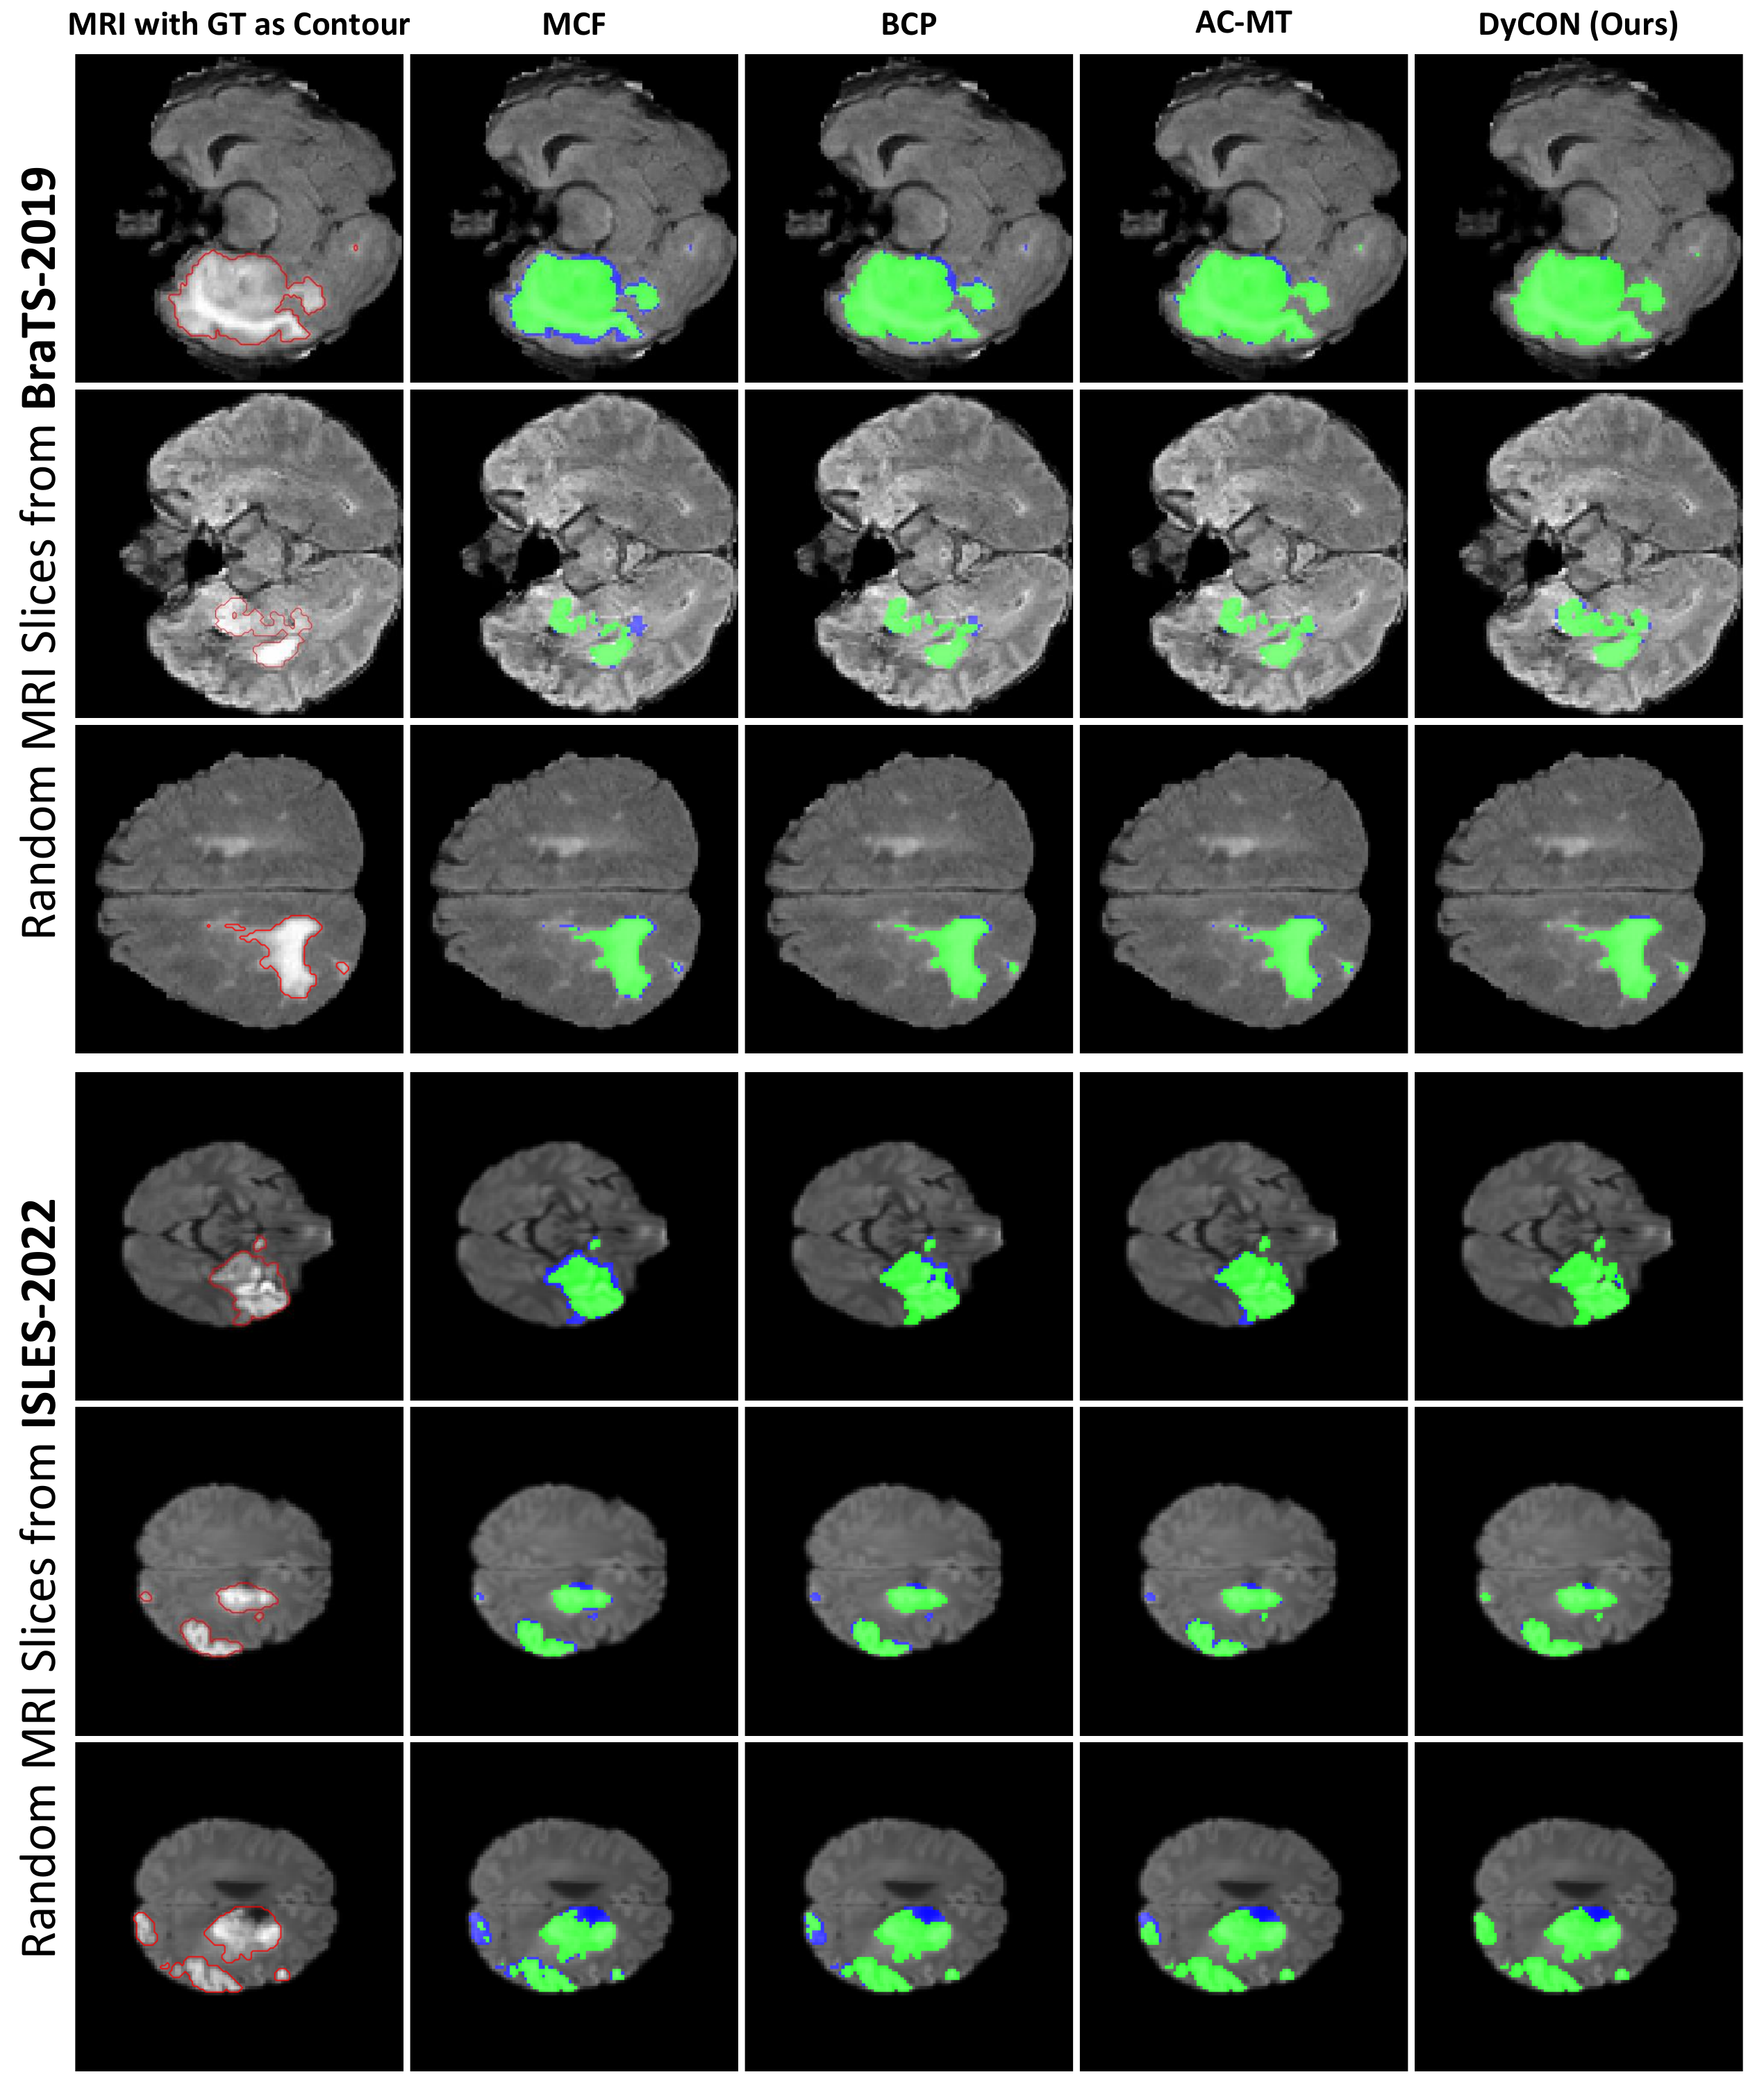}
    \caption{Comparison of brain tumor and lesion segmentation with SOTA methods. The comparison results are illustrated in terms of True Positives (green), and False Negatives (blue) in segmenting challenging lesions of MRI scans. The baseline methods struggle with detecting subtle lesion boundaries across both datasets, resulting in higher instances of FNs (blue) while DyCON effectively reduces these errors, leading to a significant number of correctly identified lesion voxels (green).}
    \label{fig:brats_and_isles_visualization}
    \vspace{-1em}
\end{figure}
\begin{figure}[!t]
    \centering
    \includegraphics[width=8.5cm]{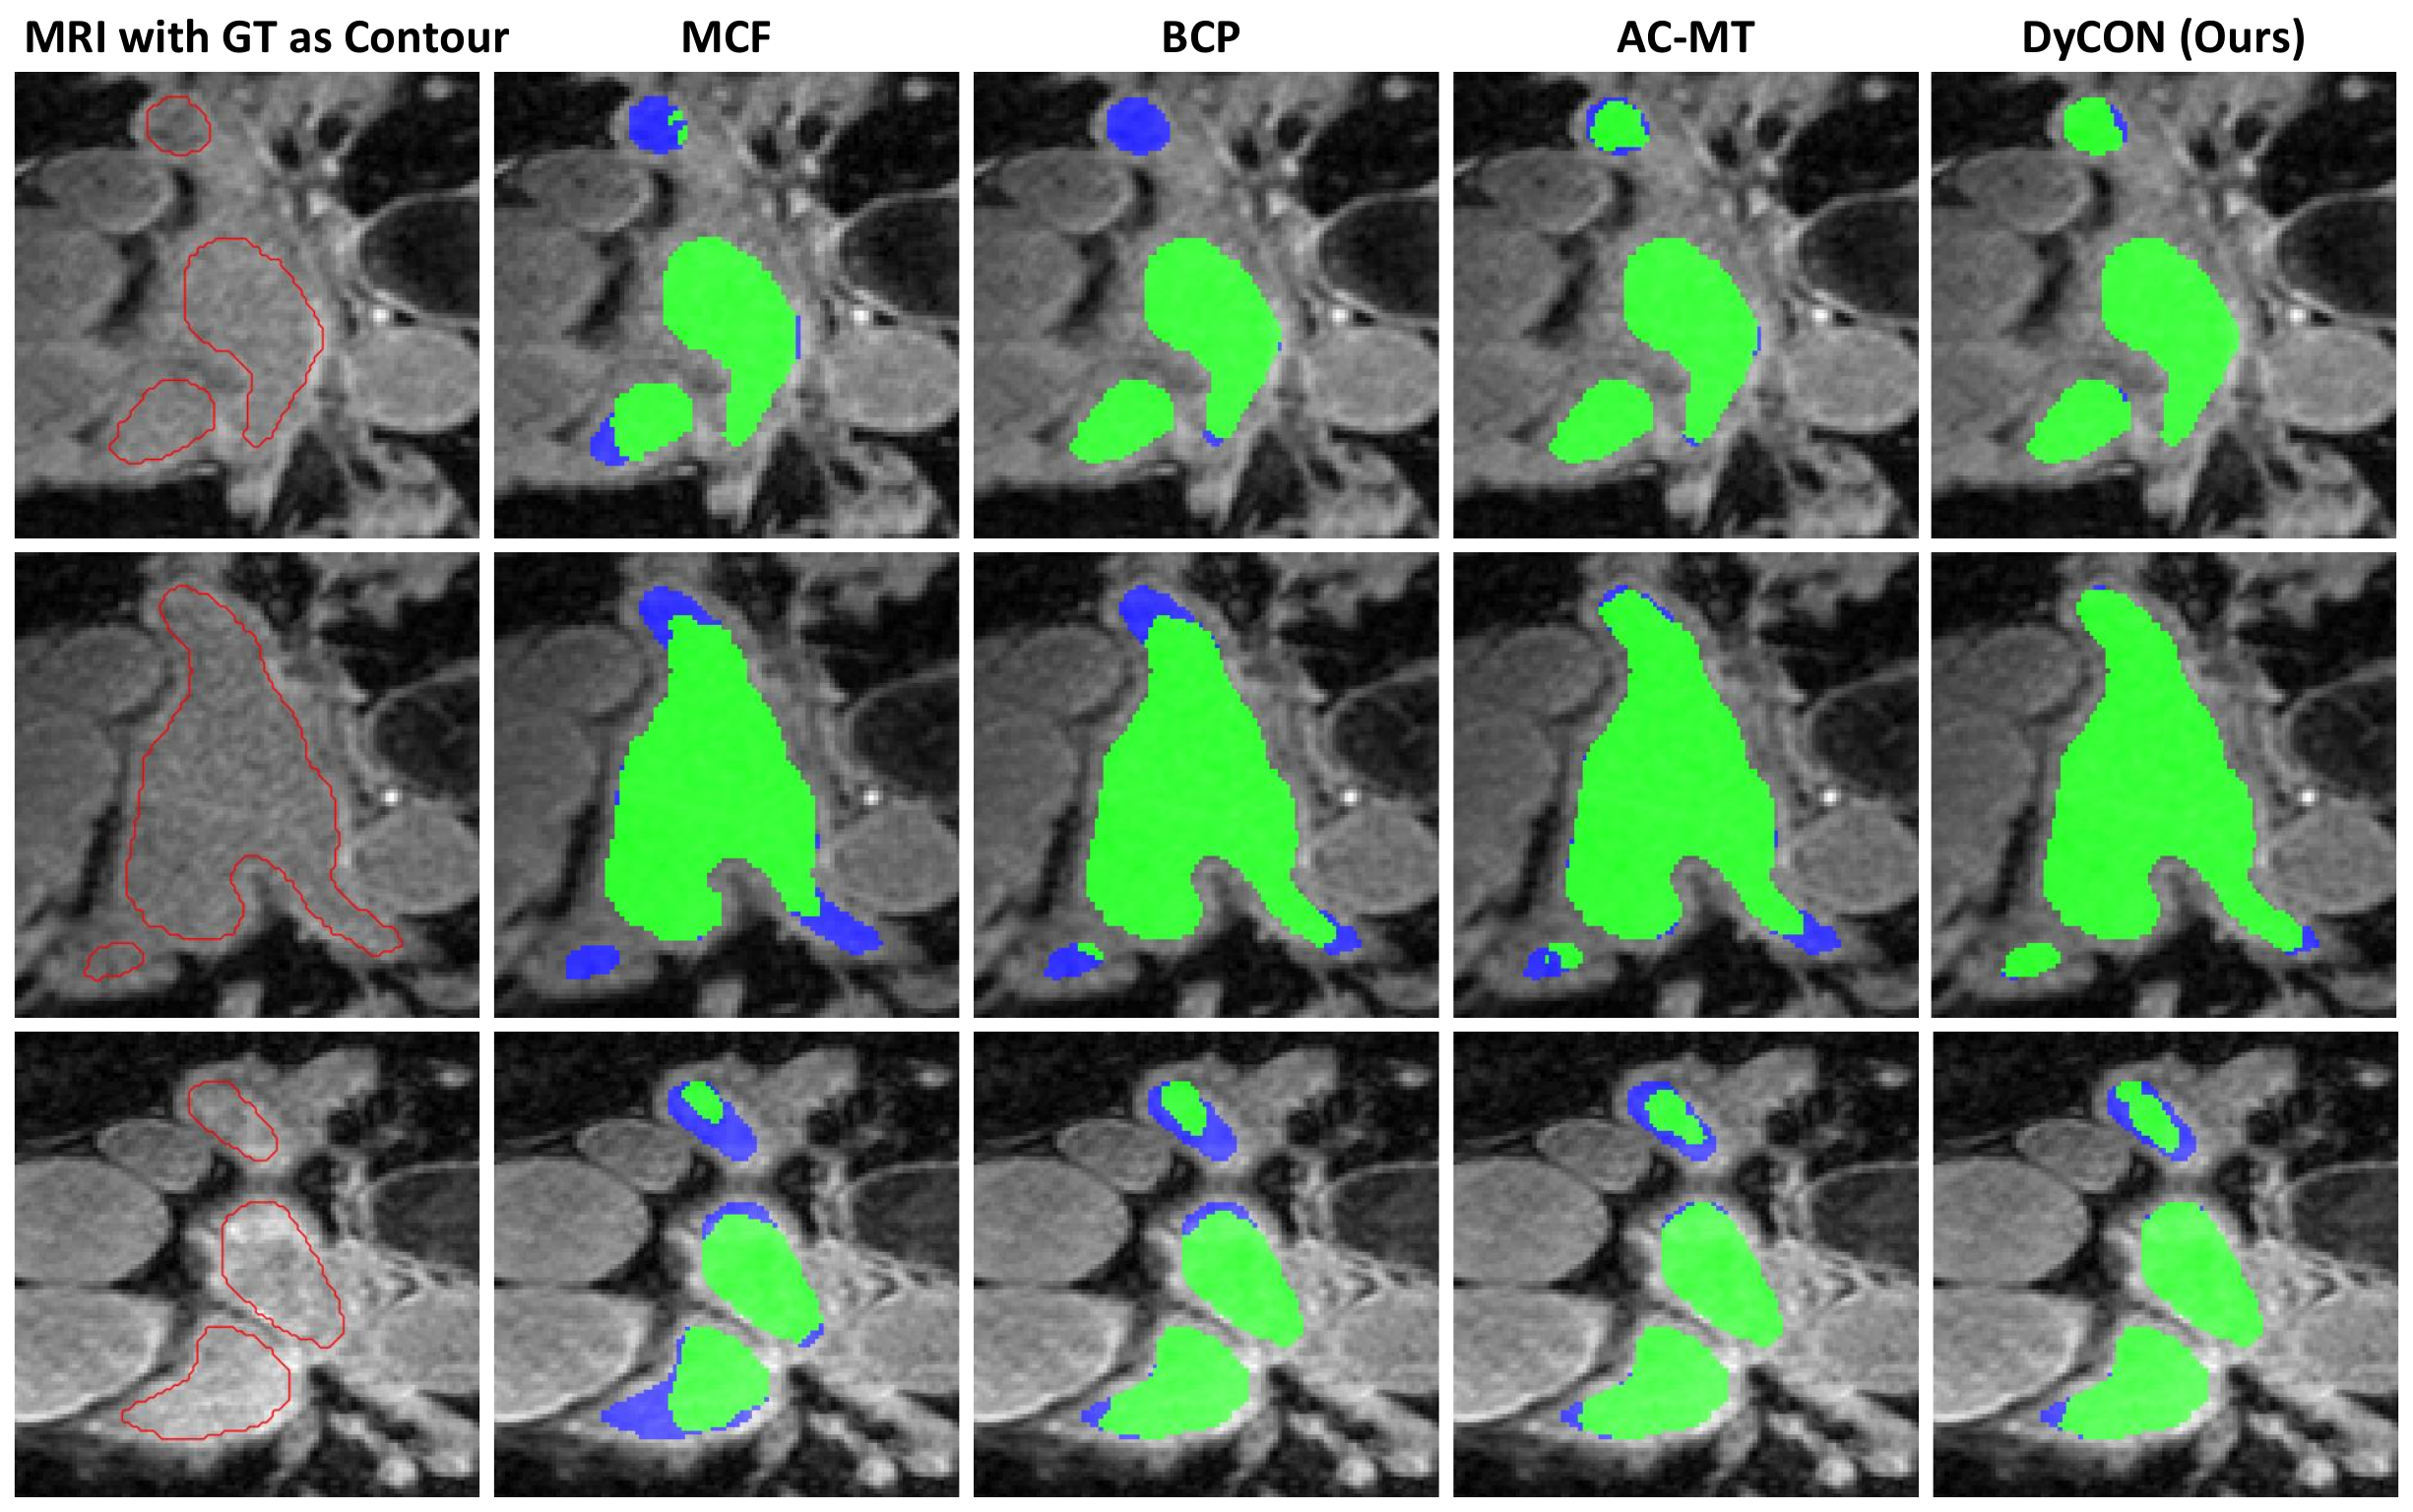}
    \caption{Comparison of challenging left atrium organ segmentation results with SOTA methods using 10\% labeled data on LA dataset. DyCON consistently produces more accurate segmentation of left atrial organs.}
    \label{fig:la_visualization}
    \vspace{-1.5em}
\end{figure}
\begin{table*}[!t]
    \centering
    \resizebox{\textwidth}{!}{
    \begin{tabular}{lcc|ccccccccccccc}
        \toprule
        \multicolumn{1}{c}{\multirow{2}{*}{Methods}} & \multicolumn{2}{c}{Average} & \multicolumn{13}{c}{Average Dice of each class using 20\% labeled data } \\ 
        \cmidrule(lr){2-3} \cmidrule(lr){4-16}
        & Dice & ASD & Sp & RK & LK & Ga & Es & Li & St & Ao & IVC & PSV & PA & RAG & LAG \\ 
        % \midrule
        % 3D-VNet~\cite{milletari:vnet} & 84.00 & 84.82 & 86.38 & 67.42 & 65.02 & 94.83 & 73.75 & 90.27 & 84.19 & 69.85 & 63.54 & 62.60 & 65.02 & 76.28 & 77.45 \\
        \midrule
        DHC~\cite{dhc}         & 48.6      & 10.7     & 62.8      & 69.5     & 59.2      & {\bf66.0} & 13.2      & 85.2      & 36.9      & 67.9      & 61.5     & 37.0      & 30.9      & 31.4      & 10.6 \\ 
        GA+MagicNet~\cite{ga}  & 68.4      & {\bf3.1} & 81.4      & {\bf92.4}& 90.8      & 33.5      & 53.3      & 89.1      & {\bf60.9} & 79.1      & {\bf82.1}& {\bf66.7} & 48.7      & 50.3      & {\bf61.4} \\ 
        {\bf DyCON+GA+MagicNet}& {\bf69.5} & 3.5      & {\bf88.5} & 85.9     & {\bf 92.6}& 49.6 & {\bf60.9} & {\bf90.6} & 58.7      & {\bf85.7} & 81.1     & 62.4 & {\bf51.9} & {\bf55.9} & 39.64 \\ 
        \bottomrule
    \end{tabular}
    }
    \caption{DyCON outperforms all methods in some organ classes while it remains comparable with other classes.}
    \label{tab:btcv_20p}
    \vspace{-1.5em}
\end{table*}

\section{Experiments on Multi-Organ Segmentation}
\label{sec:btcv_results}

To further assess the versatility and robustness of DyCON, we conducted additional experiments on the BTCV (Synapse) dataset for multi-organ segmentation, following the evaluation protocol established by existing SOTA methods such as DHC~\cite{dhc}, and GA~\cite{ga} combined with MagicNet~\cite{magicnet} (GA+MagicNet). The BTCV dataset encompasses segmentation tasks across various abdominal organs, each posing unique challenges, including considerable variability in organ size, shape, boundary ambiguity, and proximity to neighboring structures. Therefore, we integrated our proposed losses, UnCL and FeCL into the GA+MagicNet framework, creating the DyCON+GA+MagicNet variant. Table~\ref{tab:btcv_20p} illustrates the comparative performance of DyCON against the previous SOTA DHC and GA+MagicNet across thirteen different organ classes.

DyCON significantly surpasses GA+MagicNet, achieving new SOTA average Dice performance of \textbf{69.5\%}, attaining a +1.1\% improvement. Specifically notable improvements are observed in challenging organ classes characterized by high uncertainty and ambiguous boundaries, such as the Spleen (Sp: \textbf{88.5\%} vs. 81.4\%), Left Kidney (LK: \textbf{92.6\%} vs. 90.8\%), Gallbladder (Ga: \textbf{49.6\%} vs. 33.5\%), Esophagus (Es: \textbf{60.9\%} vs. 53.3\%), and Aorta (Ao: \textbf{85.7\%} vs. 79.1\%). These gains underscore DyCON's capability to dynamically emphasize uncertain and ambiguous boundary regions, enhancing the accuracy of segmentation outcomes in anatomically complex areas.

Although DyCON slightly increases the ASD from 3.1mm to 3.5mm compared to GA+MagicNet, the improvement in Dice scores across critical organs indicates that DyCON prioritizes precision in delineating organ boundaries over minimal surface distance discrepancies, beneficially balancing boundary sharpness and general segmentation robustness. Overall, these results reinforce DyCON's effectiveness as a versatile semi-supervised learning framework, not only for brain lesion segmentation but also extending its applicability and superior performance to complex multi-organ segmentation tasks.
